# Supplementary material for: Beyond Shadows: A Large-Scale Benchmark and Multi-Stage Framework for High-Fidelity Facial Shadow Removal
Source: arXiv:2601.19309 source file (2026-01-27)
Supplement: Supplementary file 3 [file supp3.tex]

\begin{figure*}
\centering
\includegraphics[height=.95\textheight]{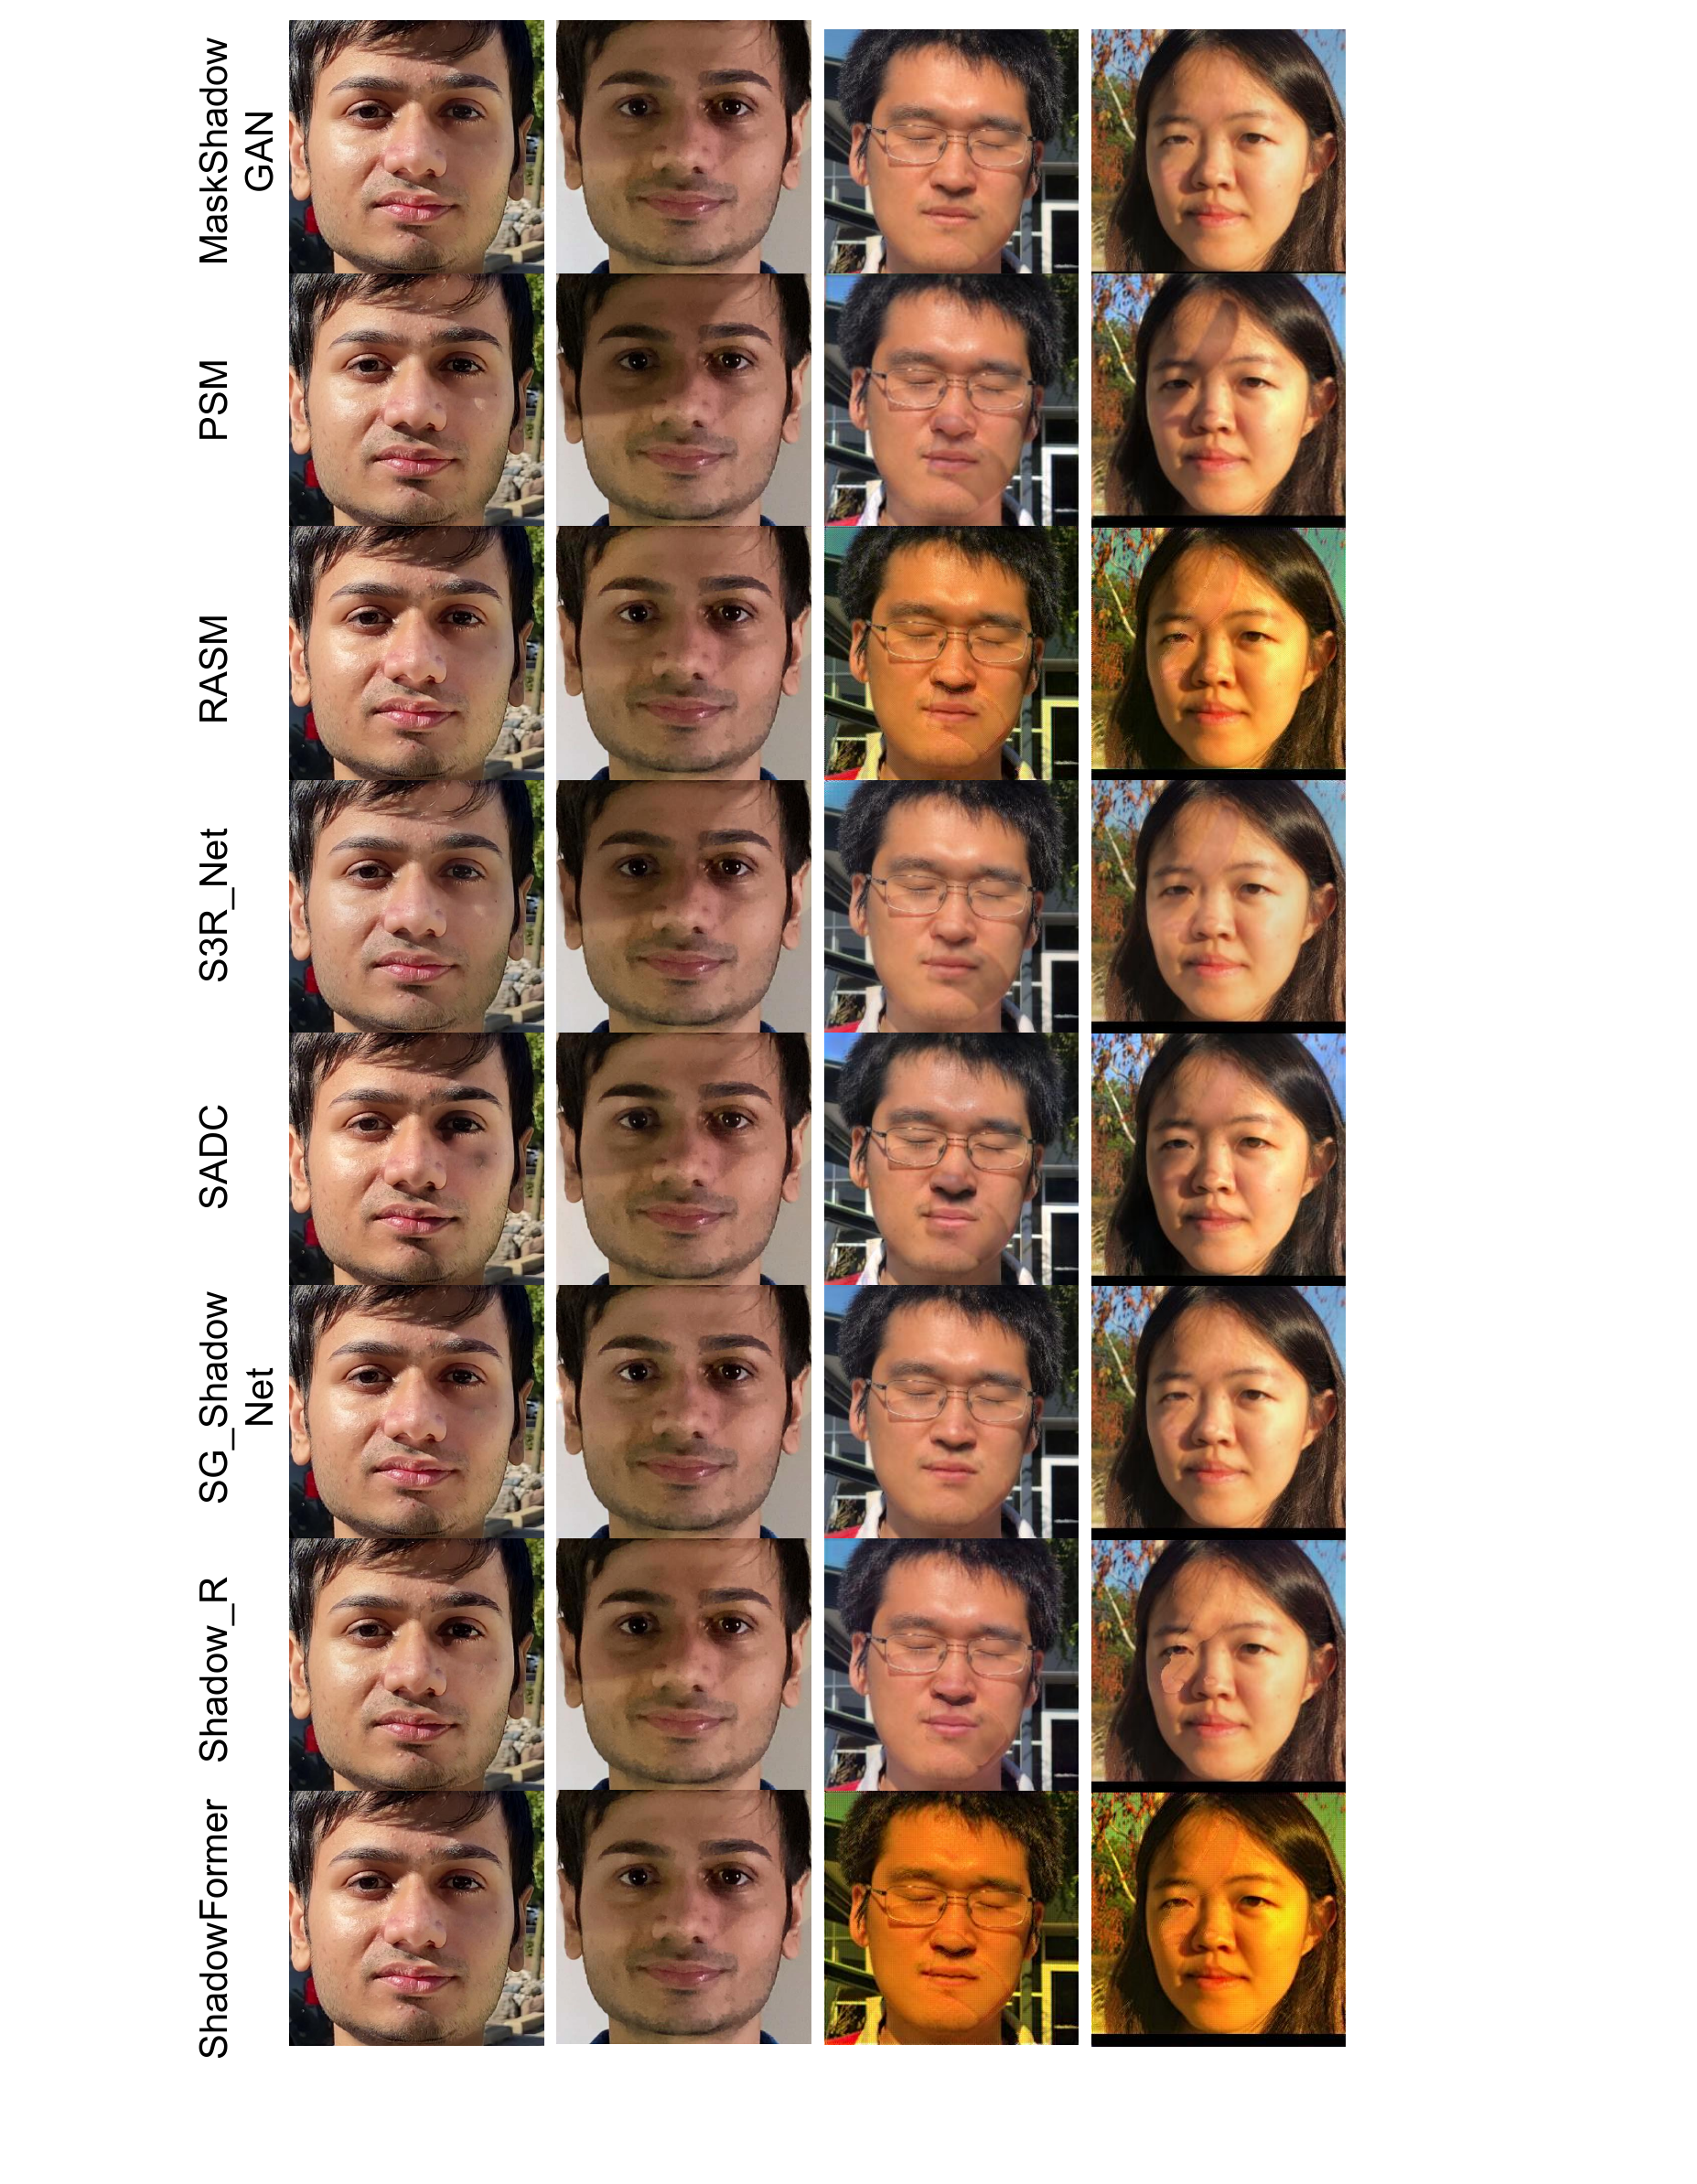}
\caption{More Visualization}
\label{supp:fig3}
\end{figure*}
